# Supplementary material for: Colloidal diffusiophoresis in crossed electrolyte gradients: experimental demonstration of an 'action at a distance' effect predicted by the Nernst-Planck equations
Source: arXiv:2311.13287 ancillary file (2023-11-23)
Supplement: Supplementary file 1 [file SM.pdf]

# Supplementary Information For: Colloidal diffusiophoresis in crossed electrolyte gradients: experimental demonstration of an 'action at a distance' effect predicted by the Nernst-Planck equations

Ian Williams,[1] Patrick B. Warren,[2,*] Richard P. Sear,[1,†] and Joseph L. Keddie[1]

[1]*School of Mathematics and Physics, University of Surrey, Guildford GU2 7XH, United Kingdom*
[2]*The Hartree Centre, STFC Daresbury Laboratory, Warrington WA4 4AD, United Kingdom*
(Dated: November 22, 2023)

## I. DESCRIPTION OF SUPPLEMENTARY MOVIES

**Supplementary Movie 1** — Experimental video showing 1 $\mu$m diameter polystyrene particles moving in orthogonal gradients of KOAc and NaCl. KOAc source is located off the top edge of the field of view. NaCl source is located off the right edge of the field of view. Magnification is 10×. Frame rate is 1 frame per second. Playback rate is 30 frames per second. Full movie duration represents 20 minutes of real time.

**Supplementary Movie 2** — Experimental arrow plot video showing velocity fields obtained from particle imaging velocimetry of the experiment shown in Supplementary Movie 1. Movie duration and frame rate are the same as Supplementary Movie 1. Each PIV cell is square of side length 45 $\mu$m.

**Supplementary Movie 3** — Simulated arrow plot video showing velocity fields predicted by the full model, incorporating the current-driven contribution to diffusiophoresis for superposed orthogonal gradients of KOAc and NaCl. The KOAc source is the top edge. The NaCl source is the right edge. Simulated region is a square of side length 3000 $\mu$m. Every tenth frame of the simulation is visualised, meaning that frames in the movie are separated by 0.9 s and the total movie duration is 6 minutes. Playback is at 15 frames per second.

**Supplementary Movie 4** — Simulated arrow plot video showing velocity fields predicted by the local model for superposed orthogonal gradients of KOAc and NaCl. The KOAc source is the top edge. The NaCl source is the right edge. Simulated region is a square of side length 3000 $\mu$m. Every tenth frame of the simulation is visualised, meaning that frames in the movie are separated by 0.9 s and the total movie duration is 6 minutes. Playback is at 15 frames per second.

**Supplementary Movie 5** — Experimental video showing 1 $\mu$m diameter polystyrene particles moving in orthogonal gradients of TBAB and NaCl. TBAB source is located off the top edge of the field of view. NaCl source is located off the right edge of the field of view. Magnification is 10×. Frame rate is 1 frame per second. Playback rate is 30 frames per second. Full movie duration represents 20 minutes of real time.

**Supplementary Movie 6** — Experimental video showing 1 $\mu$m diameter polystyrene particles moving in orthogonal gradients of KCl and KOAc. KCl source is located off the top edge of the field of view. KOAc source is located off the right edge of the field of view. Magnification is 10×. Frame rate is 1 frame per second. Playback rate is 30 frames per second. Full movie duration represents 20 minutes of real time.

**Supplementary Movie 7** — Experimental video showing 1 $\mu$m diameter polystyrene particles moving in orthogonal gradients of KCl and NaCl. KCl source is located off the top edge of the field of view. NaCl source is located off the right edge of the field of view. Magnification is 10×. Frame rate is 1 frame per second. Playback rate is 30 frames per second. Full movie duration represents 20 minutes of real time.

**Supplementary Movie 8** — Experimental video showing 1 $\mu$m diameter polystyrene particles moving in a microfluidic device containing two hydrogels containing no salts. Hydrogels are located off the top and right edges of the field of view. Experimental protocol is identical to that followed when hydrogels contain salt. Magnification is 10×. Frame rate is 1 frame per second. Playback rate is 30 frames per second. Full movie duration represents 20 minutes of real time.

* patrick.warren@stfc.ac.uk
† r.sear@surrey.ac.uk

## II. LOCATING FIELD OF VIEW USING COMPOSITE IMAGES

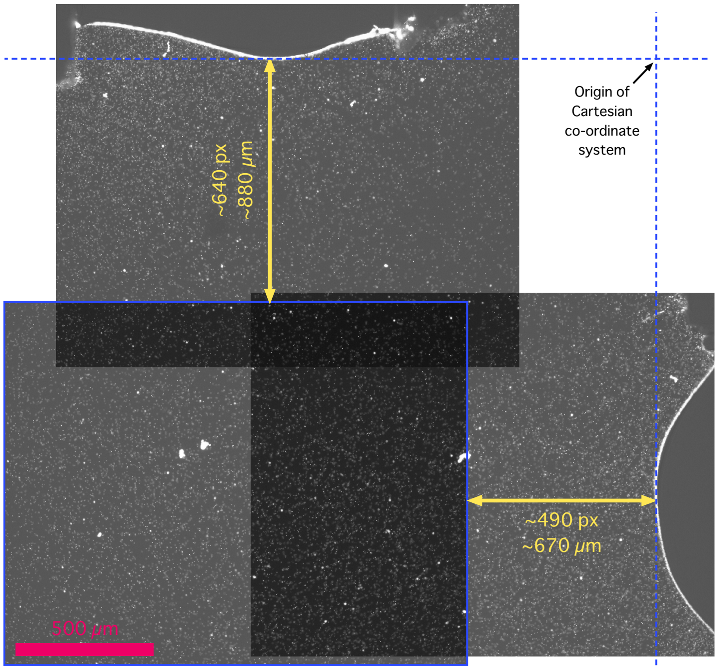


FIG. 1. Example composite image built from multiple fluorescence micrographs and used to estimate the distance between hydrogel sources (dark regions at top and right) and the field of view used for data acquisition (blue box). A Cartesian co-ordinate system is defined is normal distances from lines drawn at the edge of each hydrogel source. The location where these perpendicular lines intersect in the top right is defined as the origin.

In experiments with crossed gradients of two salts, the microscope field of view does not include either hydrogel source during data acquisition. The field of view is manually located at approximately the location of orthogonal intersection of the two gradients. As this process is manual, the exact distance between each source and the field of view differs between experiments, and it is important to estimate these distances individually for each experiment.

Immediately following the 20 minute experimental duration, the microscope field of view is translated in order to acquire additional images that include part of each hydrogel source and part of the original field of view. A composite image is then created using large, stationary particle clusters to align the final frame of the experimental video and the additional images including the hydrogel sources. An example of such a composite image is shown in Fig. 1. The approximate distance between the closest point of each hydrogel source and the edge of the experimental field of view (blue box in Fig. 1) is found, and this is used to convert co-ordinates in the experimental data into distances from the electrolyte sources. The origin of our Cartesian co-ordinate system based on distances from the sources is shown in the top right of the composite image.

## III. ONE DIMENSIONAL DIFFUSIOPHORESIS: ADDITIONAL VELOCITY PROFILES

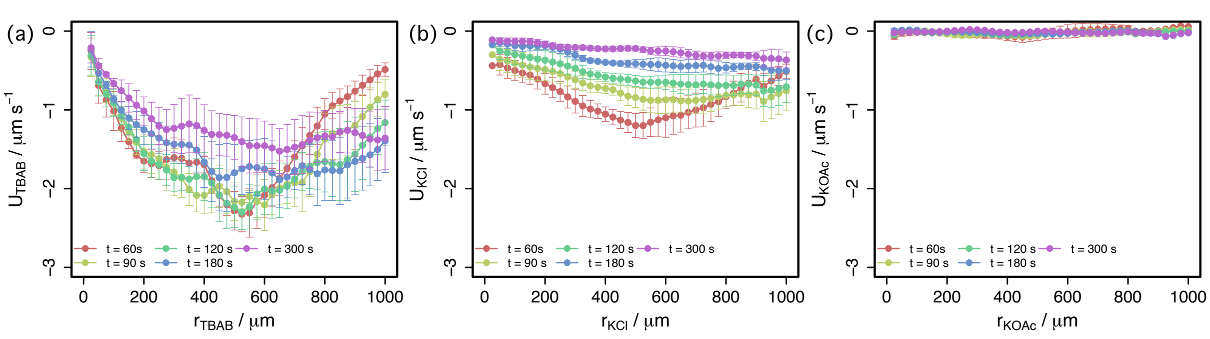


FIG. 2. Average DP velocity towards/away from hydrogel source containing (a) 130 mM TBAB, (b) 130 mM KCl, and (c) 130 mM KOAc as a function of distance from source, measured in experiments. Colour indicates time elapsed between loading the colloidal suspension into the microfluidic device and data acquisition. Each data set is the average of three repeated experiments. Error bars indicate the standard error in the mean.

Figure 2 shows experimental measurements of average diffusiophoretic velocity towards or away from the electrolyte source as a function of distance from the source in experiments with a single, 1-dimensional electrolyte gradient. Data are averaged over three repeated experiments and error bars represent the standard error in the mean. Points and lines are coloured according to the time elapsed between loading the colloidal sample into the microfluidic device and making the measurement. The main article focused on the time-dependence of the velocity profile measured in gradients of NaCl [Fig. 2 (a) of the main text], so here we present similar visualisations of the behaviour measured in gradients of (a) TBAB, (b) KCl, and (c) KOAc. In the case of KOAc, (c), the velocity profiles at all times are approximately zero, and therefore the data appear overlayed.

## IV. TWO DIMENSIONAL DIFFUSIOPHORESIS: KOAC CROSSED WITH NACL — TIME EVOLUTION OF VECTOR FIELDS

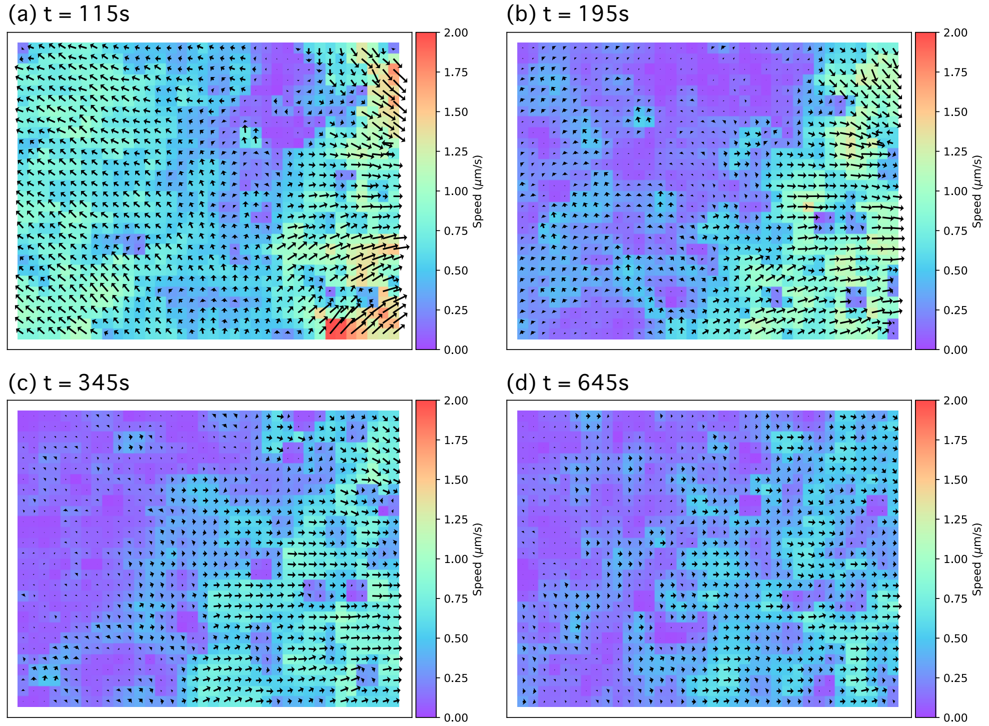


FIG. 3. Experimentally measured velocity fields in orthogonal concentration gradients of KOAc and NaCl at (a) $t \approx 115\,\mathrm{s}$, (b) $t \approx 195\,\mathrm{s}$, (c) $t \approx 345\,\mathrm{s}$, and (d) $t \approx 645\,\mathrm{s}$. The KOAc source is located $\sim 840\,\mu\mathrm{m}$ from the top of the field of view and the NaCl source is located $\sim 865\,\mu\mathrm{m}$ from the right of the field of view. Space between adjacent velocity vectors is $44\,\mu\mathrm{m}$.

Figure 3 shows the time evolution of the velocity field measured in orthogonal gradients of KOAc and NaCl. DP slows down as time proceeds, and becomes increasingly dominated by motion towards the NaCl source (right hand side).

## V. TWO DIMENSIONAL DIFFUSIOPHORESIS: KCL CROSSED WITH NACL

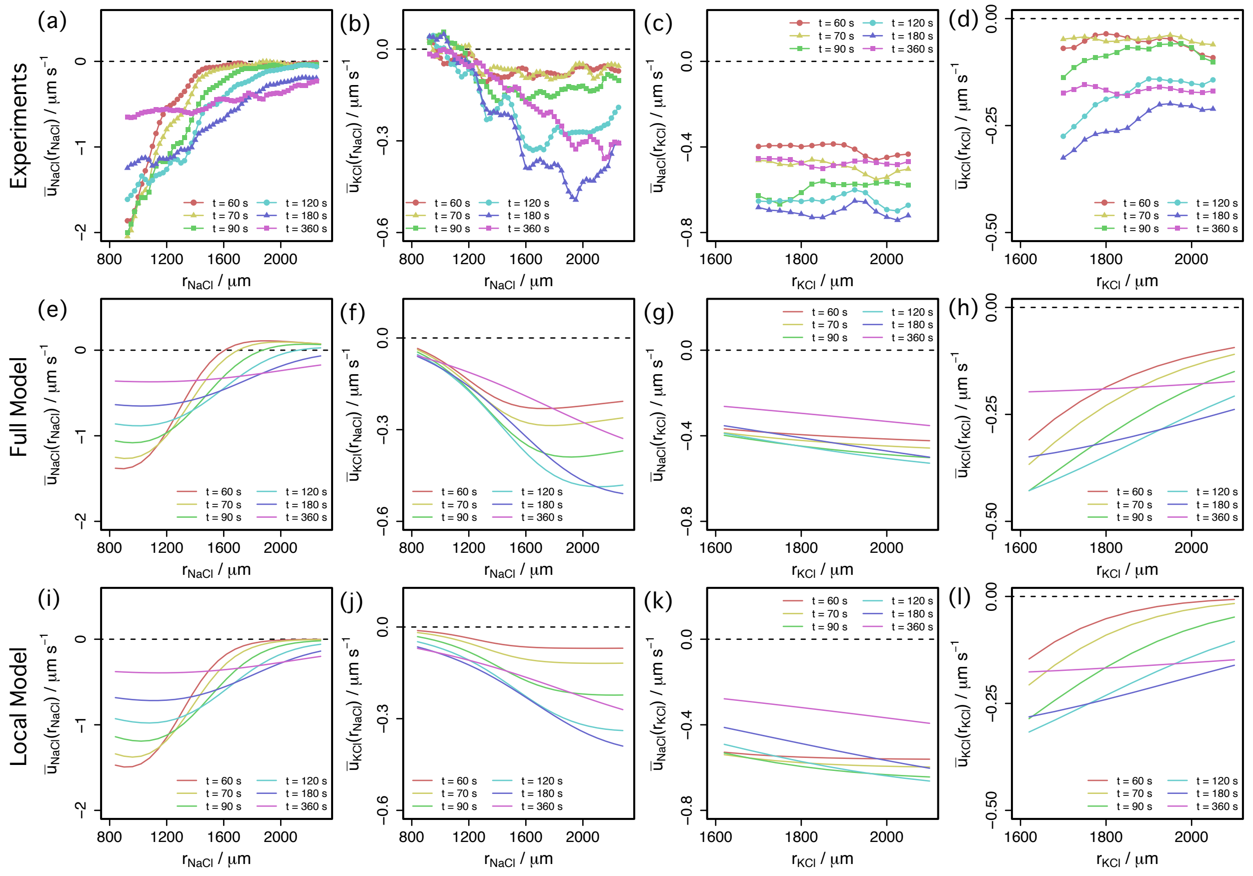


FIG. 4. KCl crossed with NaCl. Projected velocity profiles in the region for which all three experiments overlap. Colour represents time after initiation, as indicated in legends. Horizontal dashed lines indicate $U = 0$. (a-d) Experimental velocity profiles computed as an average over three repeated experiments. (e-h) Velocity profiles predicted by the full model, including the nonlocal contribution to DP. (i-l) Velocity profiles predicted by the local model. (a), (e), & (i) show $\bar{U}_{\mathrm{NaCl}}(r_{\mathrm{NaCl}})$. (b), (f), & (j) show $\bar{U}_{\mathrm{KCl}}(r_{\mathrm{NaCl}})$. (c), (g), & (k) show $\bar{U}_{\mathrm{NaCl}}(r_{\mathrm{KCl}})$. (d), (h), & (l) show $\bar{U}_{\mathrm{KCl}}(r_{\mathrm{KCl}})$.

Figure 4 shows projected average velocity profiles measured in experiments superposing a gradient of KCl with a gradient of NaCl and predicted projected velocity profiles using the full and local models. These data are qualitatively the same as those shown for TBAB crossed with NaCl and therefore are not included in the main manuscript.

## VI. TWO DIMENSIONAL DIFFUSIOPHORESIS: MODELLING NATPB CROSSED WITH NACL

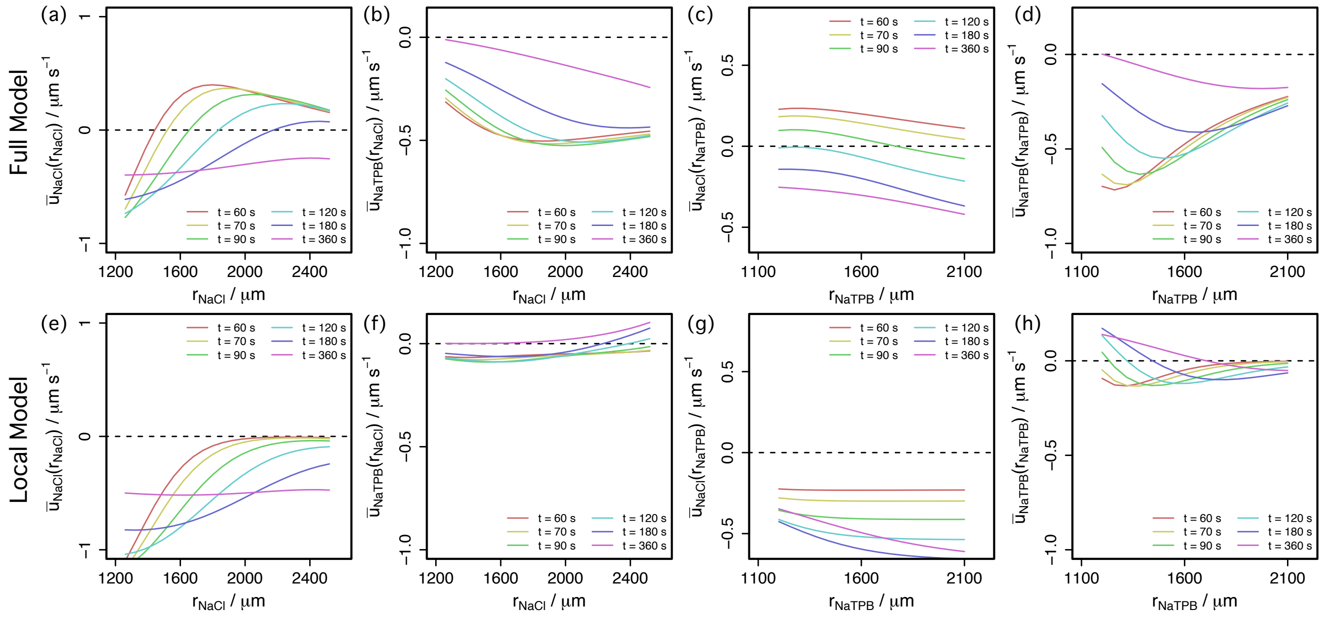


FIG. 5. Modelling NaCl superposed with NaTPB. Projected velocity profiles in the region for which all three experiments overlap. Colour represents time after initiation, as indicated in legends. Horizontal dashed lines indicate $U = 0$. (a-d) Velocity profiles predicted by the full model, including the nonlocal contribution to DP. (e-h) Velocity profiles predicted by the local model. (a) & (e) show $\bar{U}_{\mathrm{NaCl}}(r_{\mathrm{NaCl}})$. (b) & (f) show $\bar{U}_{\mathrm{NaTPB}}(r_{\mathrm{NaCl}})$. (c) & (g) show $\bar{U}_{\mathrm{NaCl}}(r_{\mathrm{NaTPB}})$. (d) & (h) show $\bar{U}_{\mathrm{NaTPB}}(r_{\mathrm{NaTPB}})$.

Figure 5 shows projected average velocity profiles predicted by modelling superposed orthogonal gradients of sodium tetraphenylborate (NaTPB) and sodium chloride (NaCl). NaTPB has $\beta = 0.4$ meaning that it drive oppositely direction chemiphoresis and local electrophoresis of particles with $\zeta = -50\,\mathrm{mV}$, but that these two contributions do not cancel one another and a net down-gradient DP should be observed in a 1d NaTPB gradient. However, modelling shows that even this imperfect cancellation is sufficient that the full model (a-d) shows qualitatively different projected velocity profiles to the local-only model (e-h). In principle, signatures of the current-driven contribution to DP should be observable in experiments using NaTPB. However, it is found that NaTPB inhibits the ability of the PEG-DA precursor solution to form a hydrogel, rendering our method of gradient generation inappropriate for use with NaTPB.

## VII. NATURAL CONVECTION DRIVEN BY GRADIENTS IN MASS DENSITY DUE TO GRADIENTS IN SALT CONCENTRATION

Concentration gradients are necessarily gradients in mass density. A 100 mM NaCl solution has a mass density approximately $4\,\mathrm{kg\,m^{-3}}$ higher than that of pure water [1]. This drives fluid flow by natural convection. The gradients established in our experiments are horizontal with respect to gravity. For a horizontal gradient there is no threshold value of the Rayleigh number for the onset of convection [2–6]. This is different from vertical gradients, for which there is a threshold value below which convection does not occur [7]. For horizontal gradients, the convection speed goes continuously to zero as the driving force for convection tends to zero. Consequently, it is not possible to completely eliminate fluid flows due to density-driven convection in experiments using a horizontal concentration gradient.

In a sealed system, fluid flow due to convection is height dependent, with flow typically circulating in opposite directions in the top and bottom halves of the channel [2, 8]. In our experiments, we would therefore expect to see particles advected in a circulating convective flow moving in different directions at different heights. This was observed in early preliminary experiments using much thicker devices of height $h \approx 300\,\mu$m, and motivated the development of thinner devices constructed using double-sided tape of thickness $h \approx 50\,\mu$m. Convection is very sensitive to system height. In linear gradients it scales as $h^3$ [2, 8]. In our thinner devices we observe little evidence of convection driven flows.

We can estimate the maximum convection speed, using a simple model of a uniform one-dimensional horizontal gradient [2, 8]. This predicts a maximum speed of approximately $10^{-2}(gh^3)(\Delta\rho/L)$, for $g$ the acceleration due to gravity, $h \approx 50\,\mathrm{\mu m}$ the fluid height, $\eta \sim 10^{-3}$ Pa s the viscosity, $\Delta\rho \approx 4\,\mathrm{kg\,m^{-3}}$ the mass density difference due to an approximately 100 mM salt concentration difference, and $L \approx 1\,\mathrm{mm}$ the horizontal system size. Putting numbers in the formula we estimate that the maximum convection speed is less than $0.1\,\mathrm{\mu m\,s^{-1}}$. This maximum is at least five times smaller than the nonlocal diffusiophoresis speeds we observe, and it is worth noting that our clearest observations of nonlocal diffusiophoresis are in regions where there are (almost) no concentration gradients, and hence not only no local diffusiophoresis, but also no local driving force for convection.

## VIII. PARTICLE VELOCITY PROFILES WITH TWO HYDROGELS CONTAINING NO SALTS

To demonstrate that negligible particle motion is measured when salts are not present, an experiment is performed using a branched microfluidic device containing two hydrogels formed without salts. In this case, the hydrogel precursor solution contains 20% by volume PEG-DA, 2% by volume photoinitiator, and 78% by volume deionised water. Besides the absence of salt, this experiment is performed and analysed identically to the experiments described in the main article. The micrograph series acquired in this experiment is provided as Supplementary Movie 8.

This experiment with "empty" hydrogels serves as a test for a number of effects. Firstly, it demonstrates that fluid flows initiated by loading the colloidal suspension into the device have decayed during the 60 seconds it takes to load the device, seal its inlets and outlets, place it on the microscope and locate and focus the region of interest. It also tests whether the introduction of fluid swells or deforms the channel walls sufficiently to induce flows in the region of interest. Additionally, it assesses the degree to which any non-photopolymerised species that remain in the hydrogel are released into solution and affect the dynamics of particles in the region of interest.

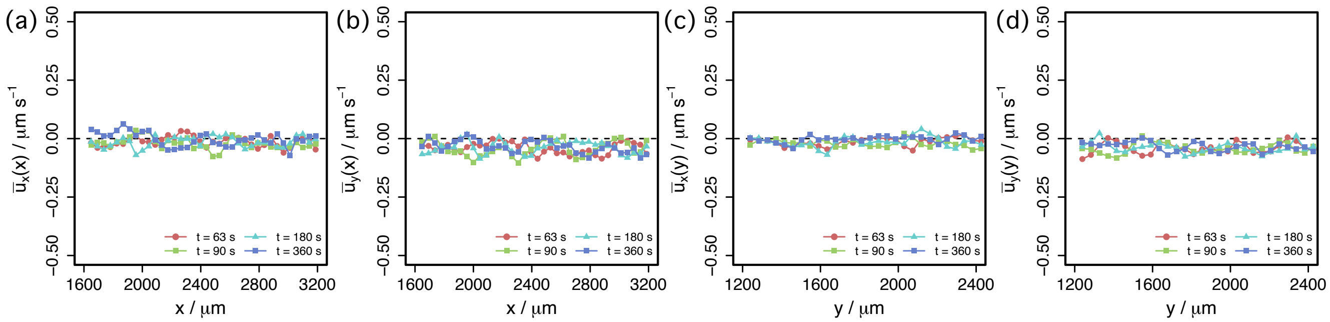


FIG. 6. Projected velocity profiles in an experiment performed in a branched microfluidic device with two hydrogels formed without salt. Colour represents time after initiation, as indicated in legends. Horizontal dashed lines indicate $U = 0$. Since hydrogels do not contain salts, co-ordinates are labeled $x$ and $y$, indicating distance from the hydrogel to the right and top of the field of view, respectively. (a) shows $\bar{U}_x(x)$. (b) shows $\bar{U}_y(x)$. (c) shows $\bar{U}_x(y)$. (d) shows $\bar{U}_y(y)$.

The empty hydrogel experiment is analysed by PIV following the same protocol as all other two-dimensional experiments. Projected velocity profiles are computed, and are shown in Fig. 6 for four different times. These data show that when salts are not present, measured particle speeds are on the scale $U \lesssim 0.1\,\mu$m/s. The $x$-components of velocities do not appear to show a prefered direction, but the $y$-components show a collective, small negative velocity, indicating upwards motion. However, such small speeds are at the limit of what can be reliably resolved in our experiments.

Therefore, we conclude that any contributions to particle motion due to residual fluid flow, or the release of non-photopolymerised species from the hydrogels are on the scale of $0.1\,\mu$m/s, and are negligible compared to diffusiophoretic speeds.

## IX. IMPACT OF INITIAL CONDITIONS ON TWO-DIMENSIONAL DIFFUSIOPHORESIS MODEL

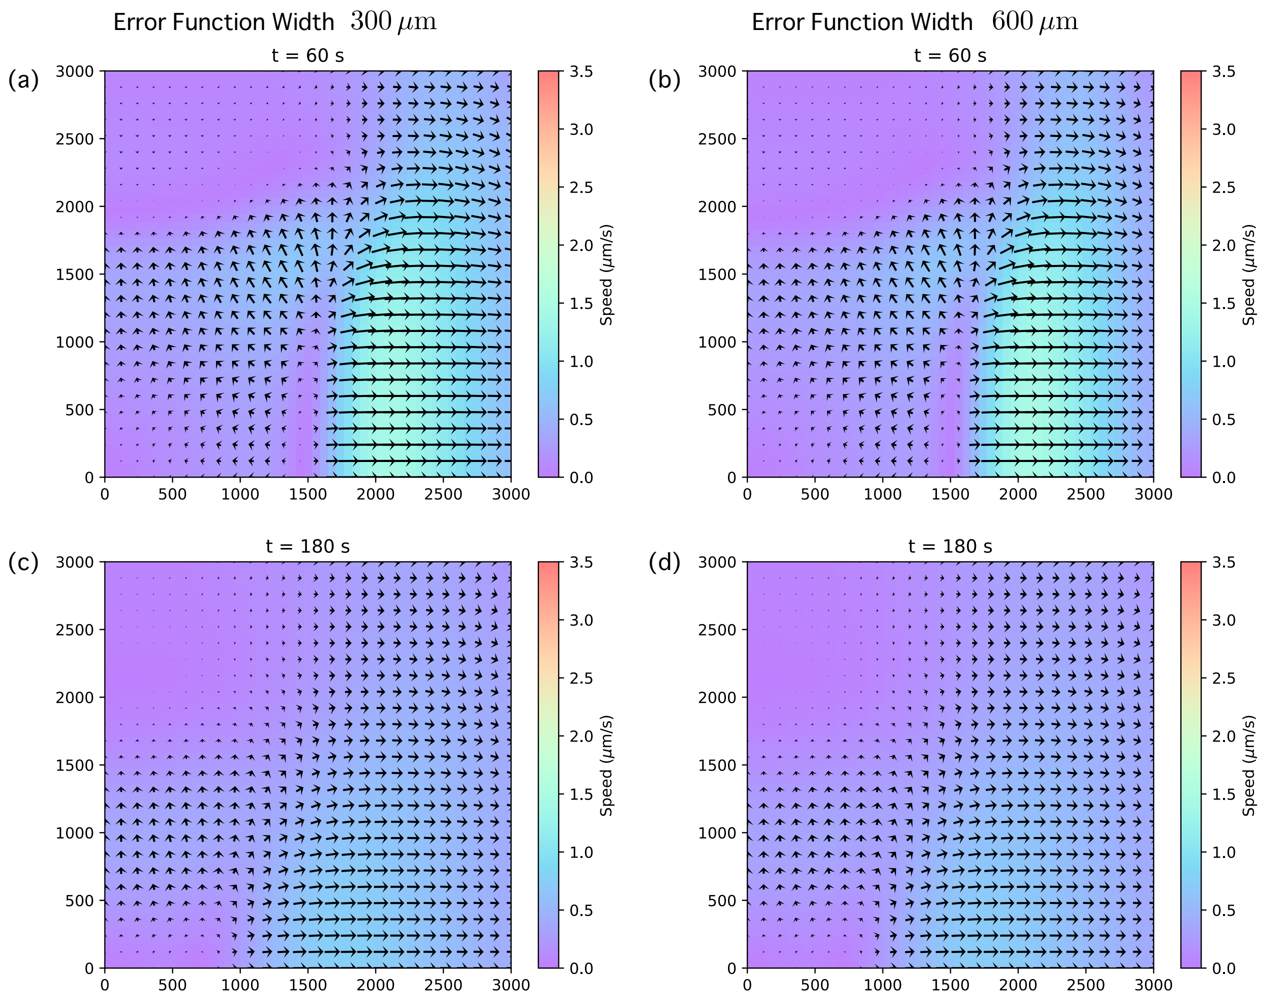


FIG. 7. Comparing simulated velocity fields in orthogonal gradients of NaCl and KOAc, incorporating all three contributions to diffusiophoresis, with different initial conditions. NaCl source is at the right and KOAc source is at the top. (a) and (c) show velocity fields at $t = 60\,$s and $t = 180\,$s when initial conditions are $300\,\mu$m wide error functions. (b) and (d) shows velocity fields at $t = 60\,$s and $t = 180\,$s when initial conditions are $600\,\mu$m wide error functions. Timescales are matched as described in the text.

The initial conditions for all two-dimensional modelling shown in the main text are error functions of width $300\,\mu$m. This width ensures that the initial concentration gradients are well-represented on the $50 \times 50$ simulatio grid. To demonstrate the impact of altering the width of these initial conditions, additional modelling has been performed for orthogonal NaCl and KOAc gradients initiated with $600\,\mu$m wide error functions.

To account for the increased width of the initial conditions, the offset time must be increased. This offset time is the time required to establish an error function concentration profile of a given width in the 1-dimensional problem described in Appendix D of the main text. As the error function concentration profile is established by diffusion, doubling the width of the error function takes four times as long. The offset time used for the simulations with $300\,\mu$m wide initial conditions is $15\,$s, based on a typical ion diffusion coefficient of $D = 1.5 \times 10^{-9}\,\mathrm{m^2\,s^{-1}}$. Therefore, the offset time required for simulations with $600\,\mu$m wide initial conditions is $60\,$s.

Supplementary Fig. 7 compares the velocity fields computed in the simulations with $300\,\mu$m wide initial conditions [(a) and (c)] and $600\,\mu$m wide initial conditions [(b) and (d)], at $t = 60\,$s [(a) and (b)] and at $t = 180\,$s [(c) and (d)]. Represented this way, the velocity fields appear very similar to each other.

Supplementary Fig. 8 shows the four projections of the velocity fields in Supplementary Fig. 7, as described in the main text, at $t = 60\,$s [(a) to (d)] and at $t = 180\,$s [(e) to (h)]. The blue lines represent $300\,\mu$m wide initial conditions

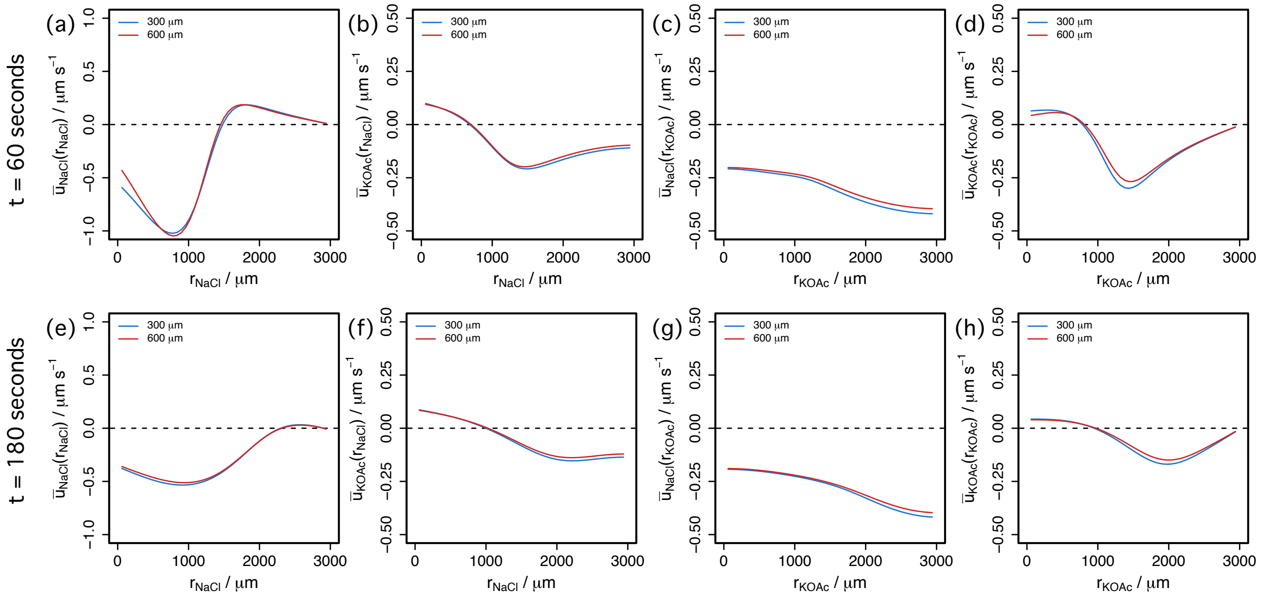


FIG. 8. Projected velocity profiles computed from velocity fields shown in Supplementary Fig. 7. (a) to (d) show projected velocity profiles at $t = 60$ s and (e) to (h) show projected velocity profiles at $t = 180$ s. Profiles computed with 300 $\mu$m wide error function initial conditions are shown in blue and profiles computed with 600 $\mu$m wide error function initial conditions are shown in red.

and the red lines show 600 $\mu$m wide initial conditions. These profiles demonstrate that when offset times are correctly accounted for, the predictions from the 2d modelling are not strongly dependent on the width of the initial conditions.

## X. DEFINING THE OVERLAPPING SUBREGION IN FOR REPEATED EXPERIMENTS

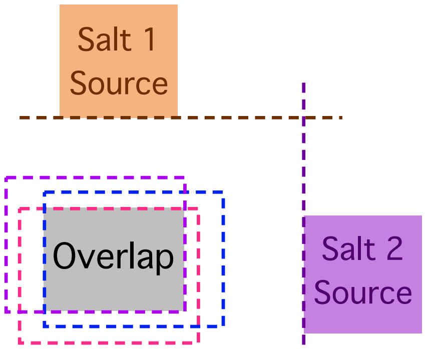


FIG. 9. The overlapping subregion. The microscope fields of view in the three experiments are in slightly different positions relative to the salt sources (purple, blue, and red dashed boxes). To combine data from repeated experiments, average velocities are computed only in the subregion for which all experiments overlap. This is indicated by the grey box.

At the start of each experiment, the microscope field of view is manually located in the region between the two salt sources. Consequently, the exact location of data acquisition with respect to the sources varies between experiments. Therefore, when combining data from multiple repeated experiments to find average particle velocity fields, we restrict out attention to the subregion for which all experiments "overlap", as illustrated in Fig. 9.

[1] J. R. Rumble, *CRC Handbook of Chemistry and Physics*, 100th ed. (CRC Press, Boca Raton FL, 2019).
[2] Y. Gu, V. Hegde, and K. Bishop, Measurement and mitigation of free convection in microfluidic gradient generators, Lab Chip **18**, 3371 (2018).
[3] S. Shin, E. Um, B. Sabass, J. T. Ault, M. Rahimi, P. B. Warren, and H. A. Stone, Size-dependent control of colloid transport via solute gradients in dead-end channels, Proc. Natl. Acad. Sci. (USA) **113**, 257 (2016).
[4] A. G. Kirdyashkin, Thermogravitational and thermocapillary flows in a horizontal liquid layer under the conditions of a horizontal temperature gradient, Int. J. Heat Mass Tran. **27**, 1205 (1984).
[5] B. Selva, L. Daubersies, and J.-B. Salmon, Solutal convection in confined geometries: Enhancement of colloidal transport, Phys. Rev. Lett. **108**, 198303 (2012).
[6] R. Birikh, Thermocapillary convection in a horizontal layer of liquid, J. Appl. Mech. Tech. Phys. **7**, 43 (1966).
[7] P. Bergé and M. Dubois, Rayleigh-bénard convection, Contemporary Physics **25**, 535 (1984).
[8] I. Williams, S. Lee, A. Apriceno, R. P. Sear, and G. Battaglia, Diffusioosmotic and convective flows induced by a nonelectrolyte concentration gradient, Proc. Natl. Acad. Sci. (USA) **117**, 25263 (2020).
